# Supplementary material for: Tree networks of real-world data: analysis of efficiency and spatiotemporal scales
Source: arXiv:2404.17829 source file (2025-02-03)
Supplement: Supplementary file 1 [file supplemental_material.pdf]

# SUPPLEMENTAL MATERIAL: TREE NETWORKS OF REAL-WORLD DATA: ANALYSIS OF EFFICIENCY AND SPATIOTEMPORAL SCALES

**Davide Cipollini**[*,1,2], **Lambert Schomaker**[1,2]
[1] Bernoulli Institute for Mathematics, Computer Science and Artificial Intelligence,
University of Groningen, Nijenborgh 9, 9747 AG Groningen, The Netherlands
[2] Cognigron - Groningen Cognitive Systems and Materials Center,
Nijenborgh 9, 9747 AG Groningen, The Netherlands
*Corresponding author: Davide Cipollini Email: d.cipollini@rug.nl

***Keywords*** Trees · Networks · Thermodynamics · Statistical physics · Machine Learning · von Neumann entropy · Specific heat

## S1 Laplacian spectrum

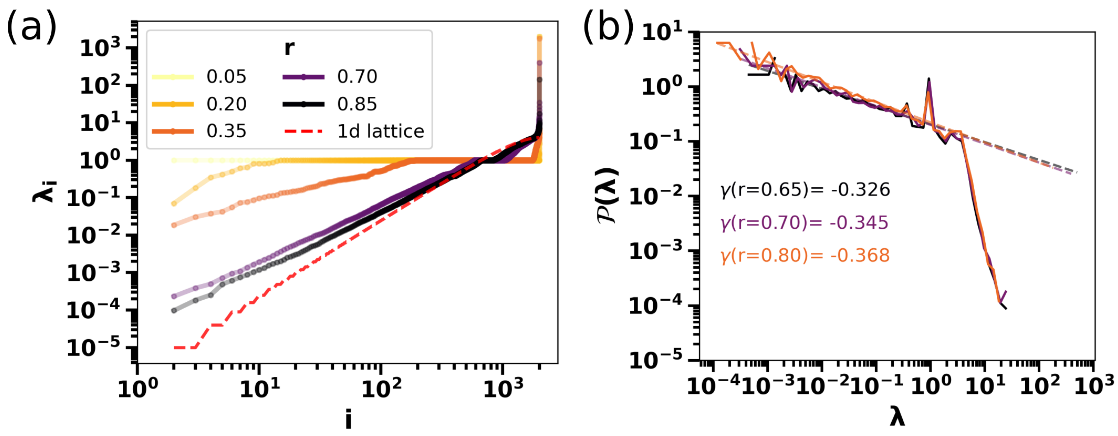


Figure S1: **Laplacian spectrum**. Panel **(a)** shows all eigenvalues for multiple values of $r$. The red dashed line indicates the limit of a 1-dimensional lattice. The greater the degeneracy in the eigenvalue spectrum the larger the peak in the specific heat (see Figure S8). For the case of the star graph $r = 0.05$ the maximum eigenvalue equals the maximum number of nodes $\lambda_{max} = 2000$. Panel **(b)** shows the spectral density, $\mathcal{P}(\lambda)$, for networks generated with selected values of $r = 0.65, 0.70, 0.80$. Note the power law behavior $\mathcal{P}(\lambda) \propto \lambda^{\gamma}$, with $\gamma \simeq -1/3$ for $\lambda \lesssim 1$. Such value of the exponent indicates a spectral dimension of $d_s = 4/3$ typical of random trees with finite variance degree distribution. We highlight the two relations discussed in the main text: (i) between the spectral dimension, $d_s$, and the power law exponent, $d_s/2 = \gamma + 1$; (ii) between the specific heat plateau, $C_0$, and the spectral dimension, $C_0 = 2d_s$ (see Figure S8). Dashed lines indicate the theoretical power law behavior with the fitted values of $\gamma$ (fit over the range $\lambda \in [10^{-3}, 5 \times 10^{-1}]$. Moreover, note the peak of the spectral density at $\lambda = 1$ due to the degeneracy of the said eigenvalue and the large number of nodes at the branch ends with degree $k = 1$. In both panels, points are averaged over 50 independent network generations from the subset of 2000 FashionMNIST samples.

## S2 Larger networks: N=4000

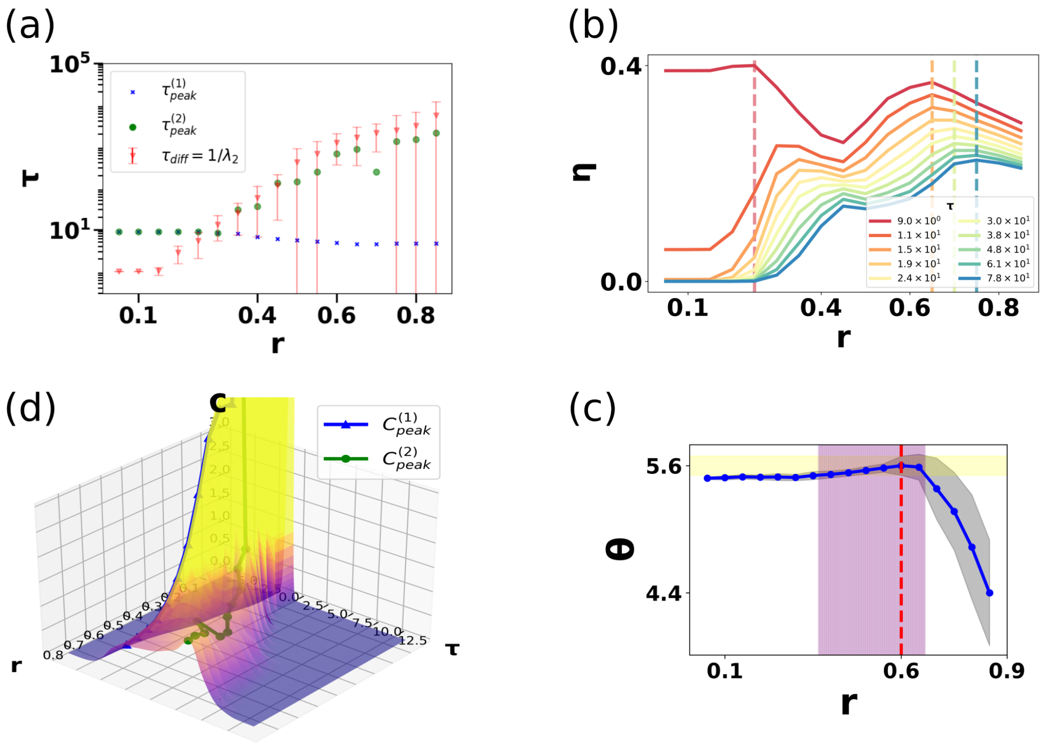

Figure S2: **MNIST - N=4000.** In **(a)** the bifurcation of $\tau_{peak}^{(1)}$ and $\tau_{peak}^{(2)}$ curves identify the $\tau$-scale relevant for the topological transition. The jump of $\tau_{peak}^{(2)}$ towards $\tau_{peak}^{(1)}$ (see at $r \sim 0.7$) is less pronounced compared to networks of 2000 nodes. In red the numerical average of the diffusion time $1/\tau_{diff} = \lambda_2$ is plotted for reference, see the main text for discussion. In **(d)** the specific heat, $C$, surface is illustrated. The $C_{peak}^{(1,2)}$ curves correspond to the specific heat values evaluated along the curves $\tau_{peak}^{(1,2)}$ in (a). In **(b)**-**(c)** the efficiencies $\eta$ and $\theta$ are plotted as a function of $r$ with the dashed lines indicating the global maxima. The $\eta$ is computed in the $\tau$-range of one order of magnitude from the $\tau$-scale indicated by the bifurcation of $\tau_{peak}^{(1,2)}$ in (a). For larger networks N=4000 optimal $r$ remains unchanged as it is a property mostly dependent on the dataset complexity. The shaded area in **(c)** spans over the two local maxima in panel **(b)** (see main text for discussion). Quantities are averaged over 50 independent simulations.

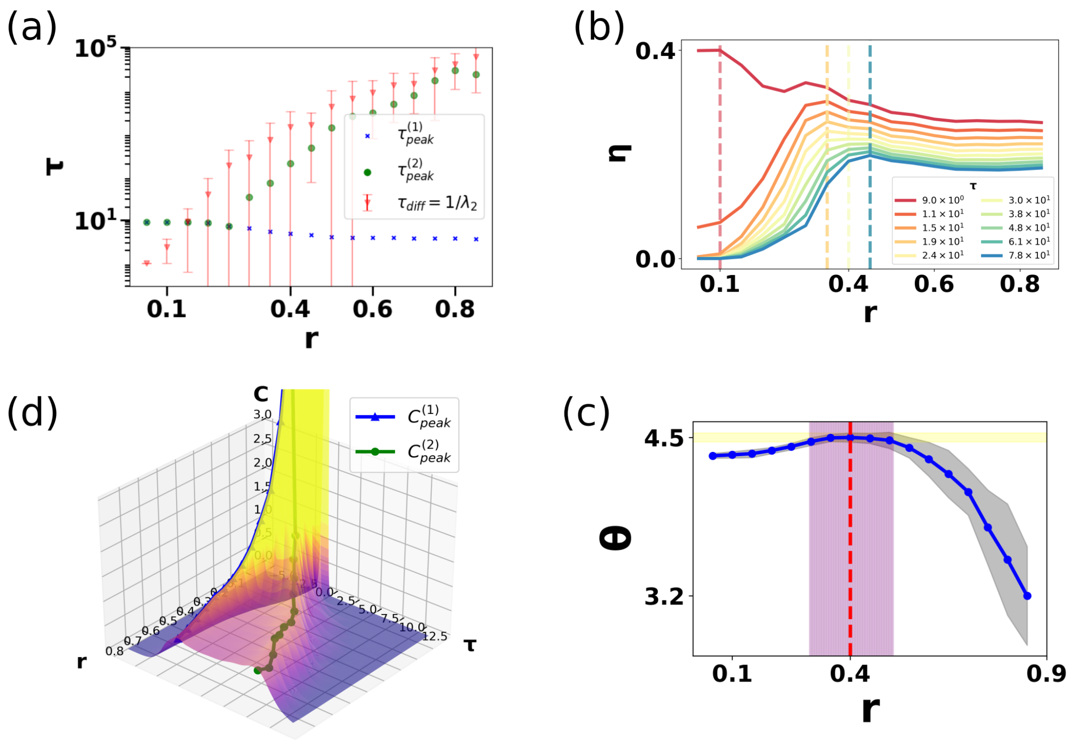


Figure S3: **FashionMNIST - N=4000.** In **(a)** the bifurcation of $\tau_{peak}^{(1)}$ and $\tau_{peak}^{(2)}$ curves identify the $\tau$-scale relevant for the topological transition. The red curve depicts the numerical average of the diffusion time $1/\tau_{diff} = \lambda_2$, see the main text for discussion. In **(d)** the specific heat, $C$, surface is illustrated. The $C_{peak}^{(1,2)}$ curves correspond to the specific heat values evaluated at $\tau_{peak}^{(1,2)}$ in (a). In **(b)-(c)** the efficiencies $\eta$ and $\theta$ are plotted as a function of $r$ with the dashed lines indicating the global maxima. The $\eta$ is computed in the $\tau$-range of one order of magnitude from the $\tau$-scale indicated by the bifurcation of $\tau_{peak}^{(1,2)}$ in (a). Note that the maxima of the efficiencies is posited at the edge of the critical value of $r \sim 0.35$ indicating the FashionMNIST as a dataset more complex than the MNIST and NIST, which does benefit from the vicinity to the phase transition. Quantities are averaged over 50 independent simulations.

# S3 $\eta$, W, U

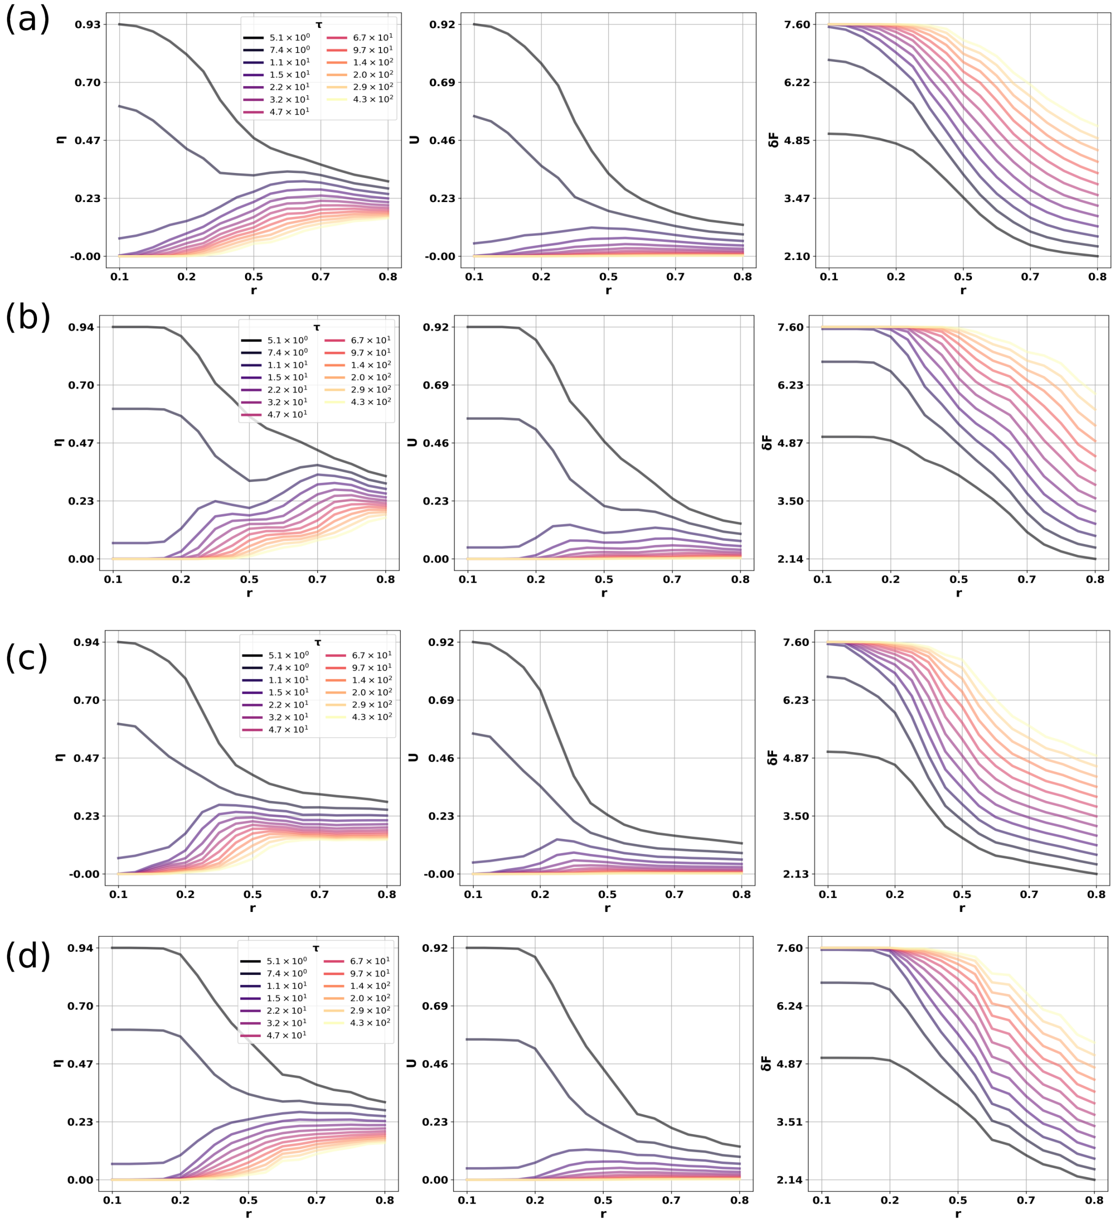

Figure S4: (a) $\eta$, $\mathbf{W}(=\delta F)$, **U for multiple resolution-scales** $\tau$. Panels **(a)-(d)** show $\eta,\ U, \delta F$ as a function of $r$ for networks of $N = 2000$ samples from the datasets NIST, MNIST, FashionMNIST, and CIFAR10 respectively. Note that $\eta$ changes concavity for $\tau < 10$. Below the mentioned resolution scale any coherence between the thermodynamic and the pattern-matching efficiency is lost. Curves are averaged over 50 independent iterations.

## S4 Von Neumann entropy and specific heat

Figures S5-S10 depict the spectral entropy, $S$, in blue, and the specific heat, $C$, in red, as a function of $\tau$ for multiple control parameter values, $r$. Y-ticks on the right axis correspond to the theoretical specific heat plateau values for: infinite 2d-lattice, $C = 1$; random trees with finite $< k^2 >$ where $k$ is the node degree, $C = 2/3$; and 1-d lattice, $C = 1/2$. Note the relation between $C$ and the spectral dimension, $d_s$, through the formula $d_s = 2C$ (see main text).

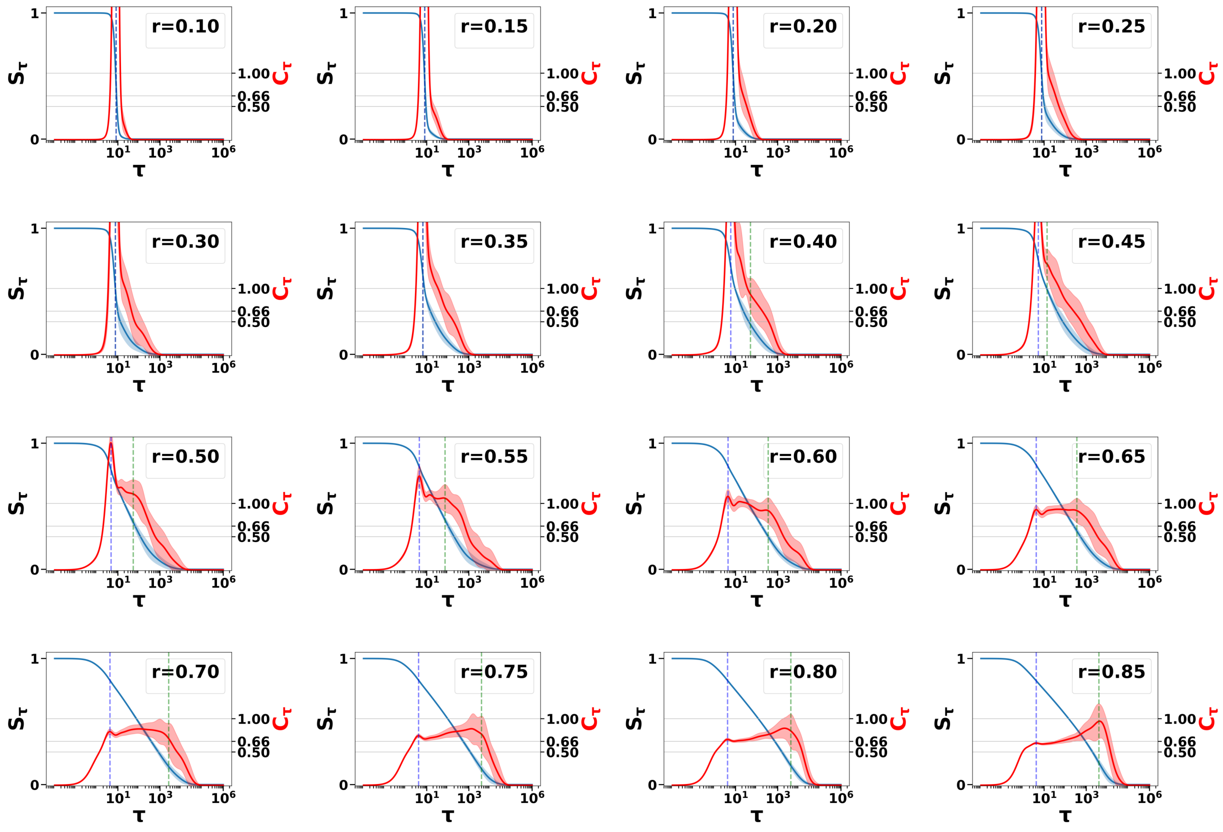

Figure S5: **Von Neumann and specific heat - NIST: 2000 samples.** The table shows the von Neumann entropy (blue) and the specific heat (red) for $r = \{0.10, ..., 0.85\}$. Vertical dashed lines indicate the peaks corresponding to $\tau^{(1)}_{peak}$ (blue) and $\tau^{(2)}_{peak}$ (green) in the main text. Shaded areas represent the standard deviation. Curves are averaged over 50 simulations.

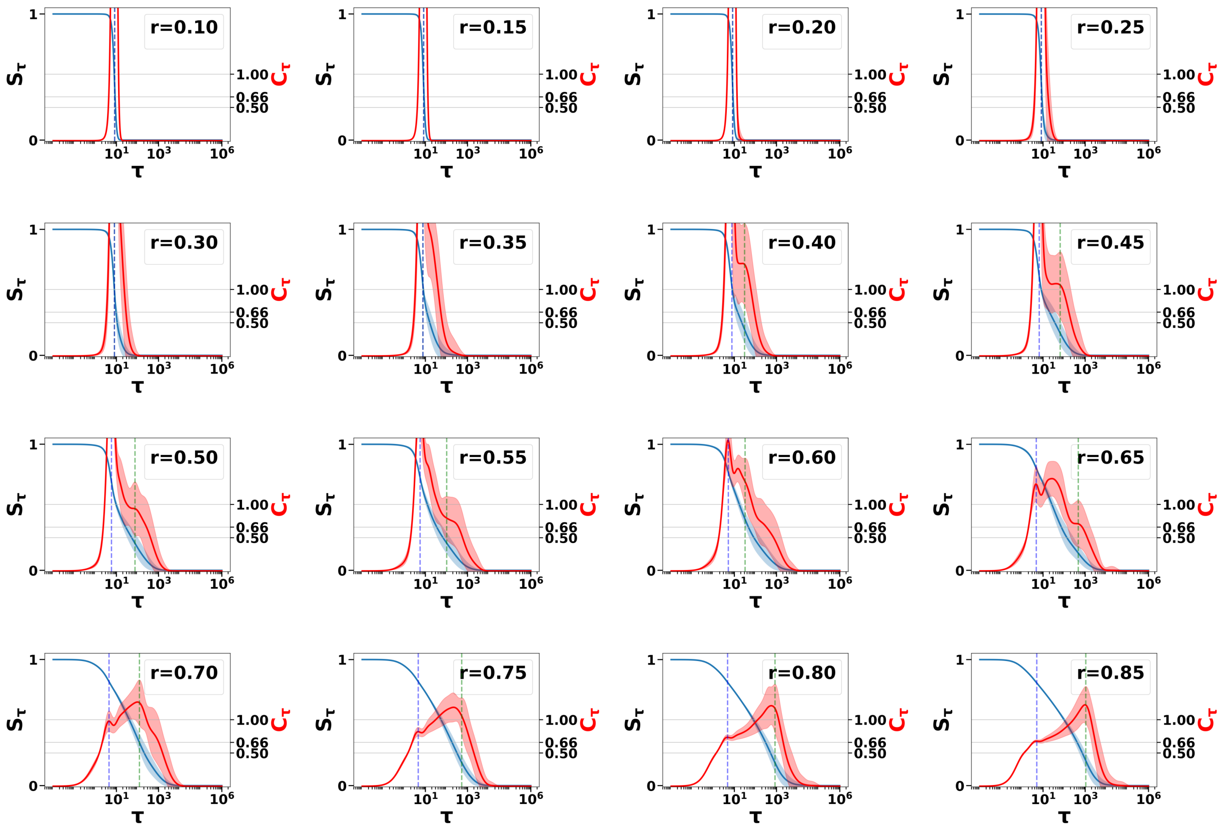


Figure S6: **Von Neumann and specific heat - MNIST: 2000 samples.** The table shows the von Neumann entropy (blue) and the specific heat (red) for $r = \{0.10, ..., 0.85\}$. Vertical dashed lines indicate the peaks corresponding to $\tau_{peak}^{(1)}$ (blue) and $\tau_{peak}^{(2)}$ (green) in the main text. Shaded areas represent the standard deviation. Curves are averaged over 50 simulations.

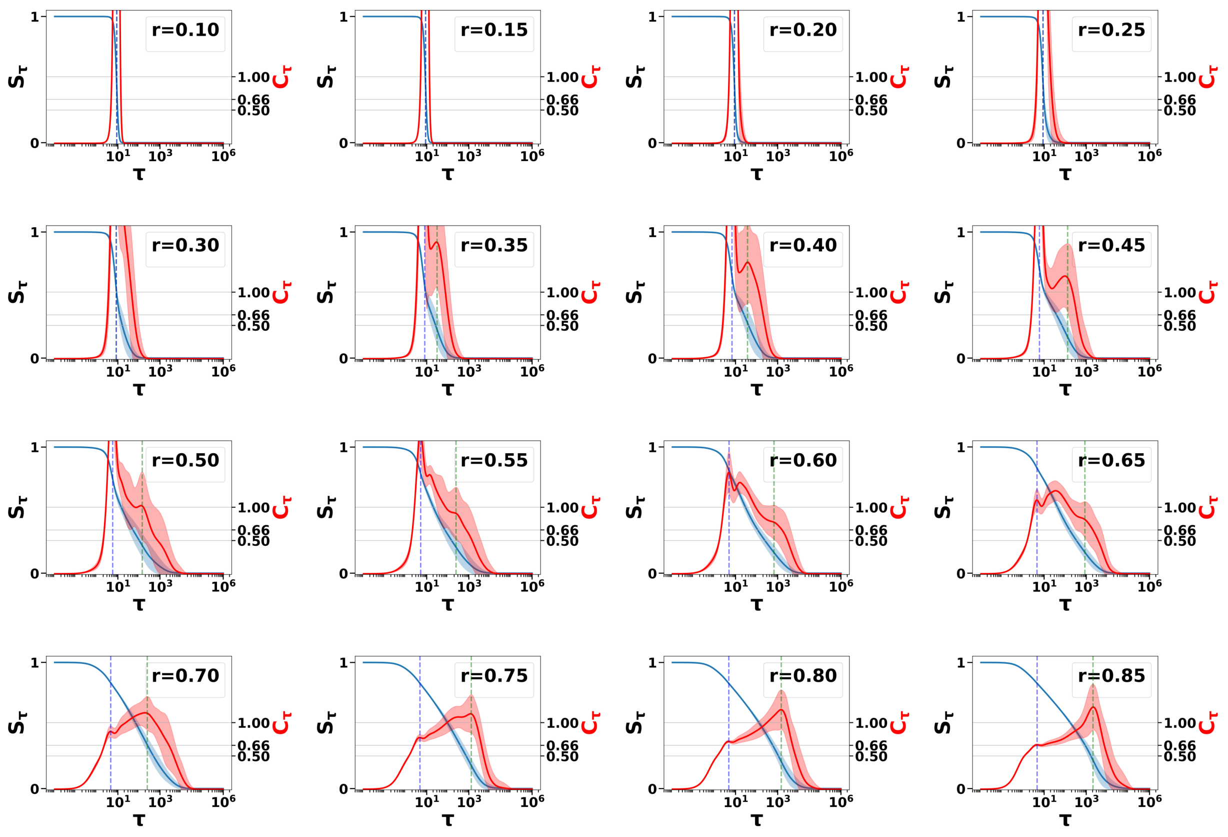


Figure S7: **Von Neumann and specific heat - MNIST: 4000 samples.** The table shows the von Neumann entropy (blue) and the specific heat (red) for $r = \{0.10, ..., 0.85\}$. Vertical dashed lines indicate the peaks corresponding to $\tau^{(1)}_{peak}$ (blue) and $\tau^{(2)}_{peak}$ (green) in the main text. Shaded areas represent the standard deviation. Curves are averaged over 50 simulations.

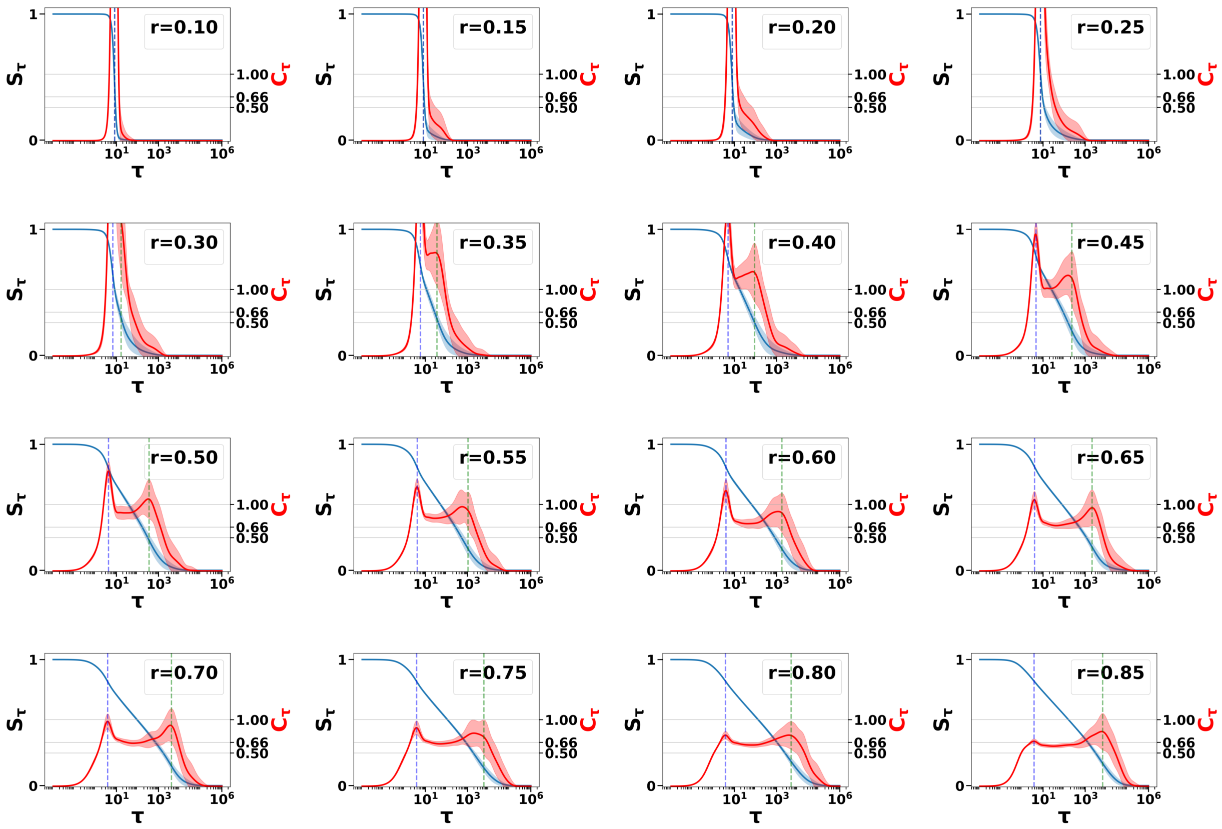

Figure S8: **Von Neumann and specific heat - FashionMNIST: 2000 samples.** The table shows the von Neumann entropy (blue) and the specific heat (red) for $r = \{0.10, ..., 0.85\}$. Vertical dashed lines indicate the peaks corresponding to $\tau^{(1)}_{peak}$ (blue) and $\tau^{(2)}_{peak}$ (green) in the main text.Shaded areas represent the standard deviation. Curves are averaged over 50 simulations.

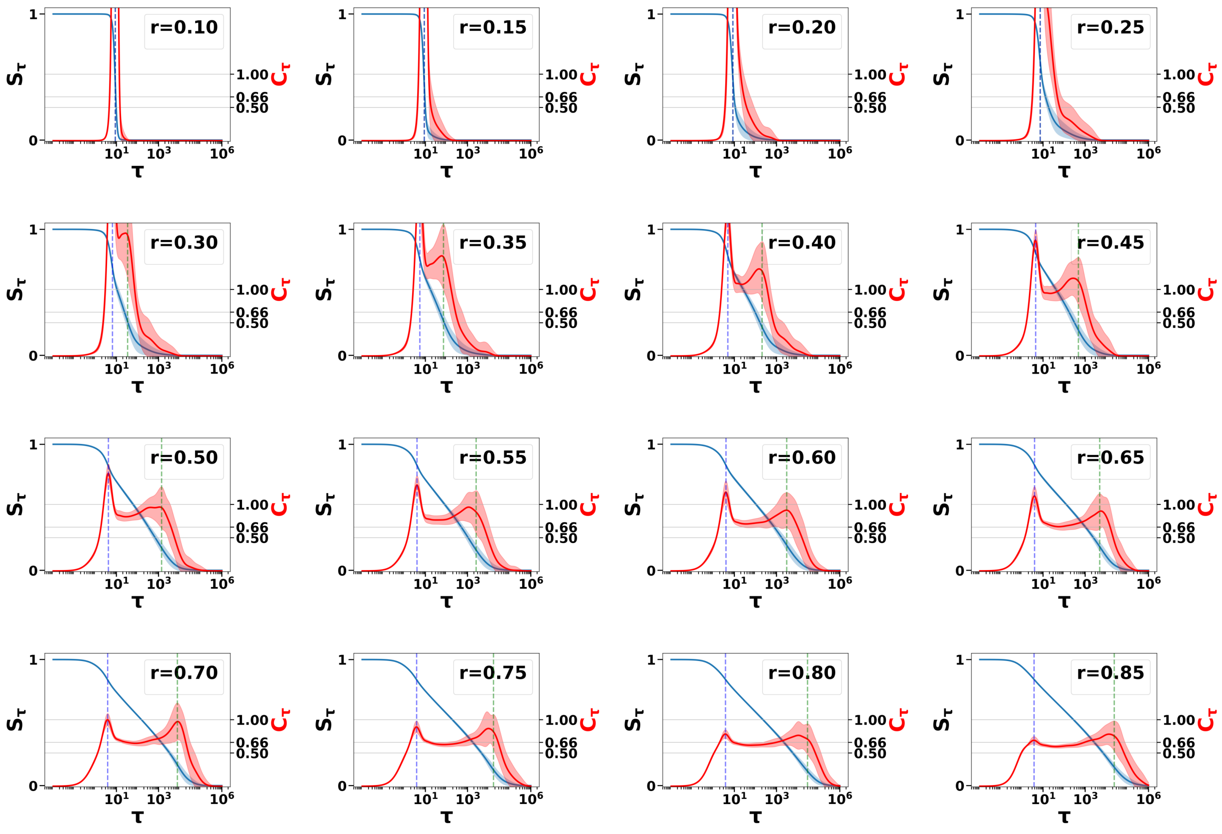


Figure S9: **Von Neumann and specific heat - FashionMNIST: 4000 samples.** The table shows the von Neumann entropy (blue) and the specific heat (red) for $r = \{0.10, ..., 0.85\}$. Vertical dashed lines indicate the peaks corresponding to $\tau_{peak}^{(1)}$ (blue) and $\tau_{peak}^{(2)}$ (green) in the main text. Shaded areas represent the standard deviation. Curves are averaged over 50 simulations.

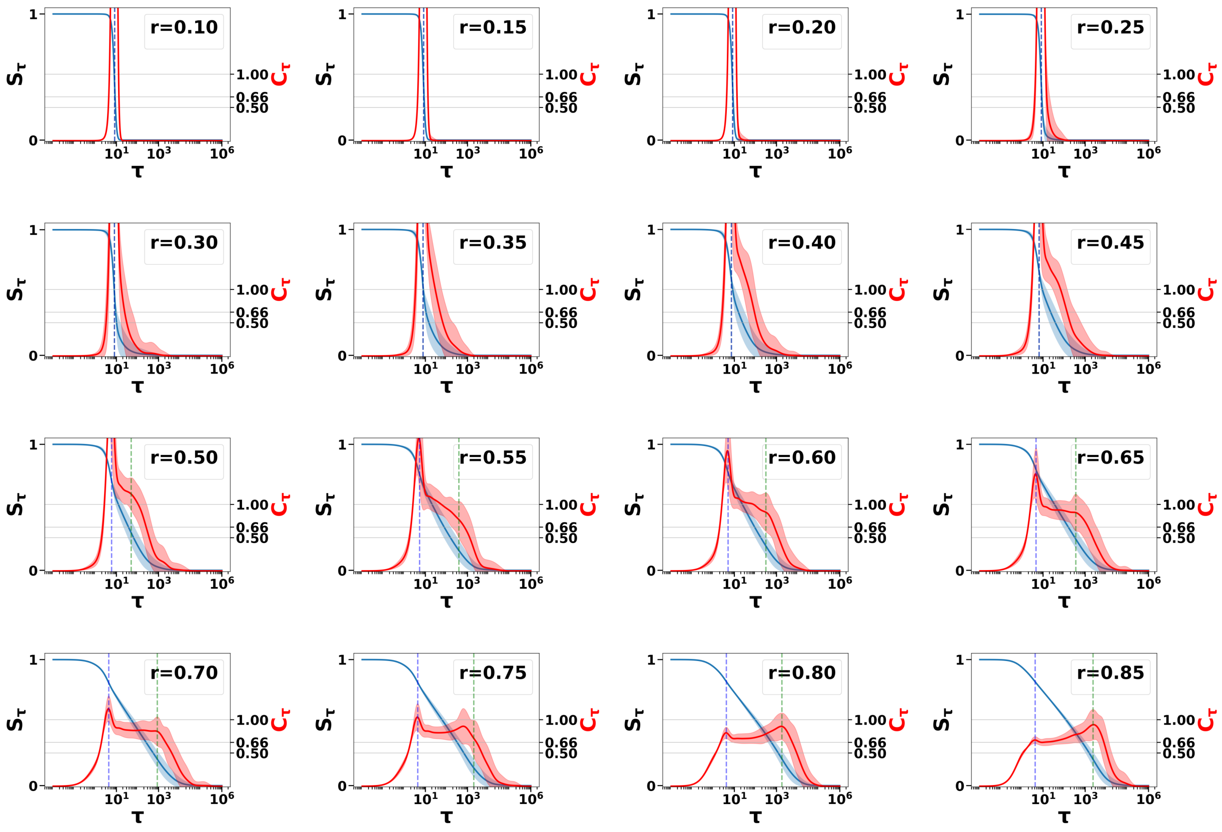


Figure S10: **Von Neumann and specific heat - CIFAR10: 2000 samples.** The table shows the von Neumann entropy (blue) and the specific heat (red) for $r = \{0.10, ..., 0.85\}$. Vertical dashed lines indicate the peaks corresponding to $\tau^{(1)}_{peak}$ (blue) and $\tau^{(2)}_{peak}$ (green) in the main text. Shaded areas represent the standard deviation. Curves are averaged over 50 simulations.

## S5 Variance analysis of F, $\delta$F, $\delta$S, $\eta$

Figure S11 shows the variance of the quantities F, $\delta F$, $\delta S$, $\eta$ for the FashionMNIST, MNIST, and NIST datasets. The peak of the variance indicates the location of the structural phase transition.

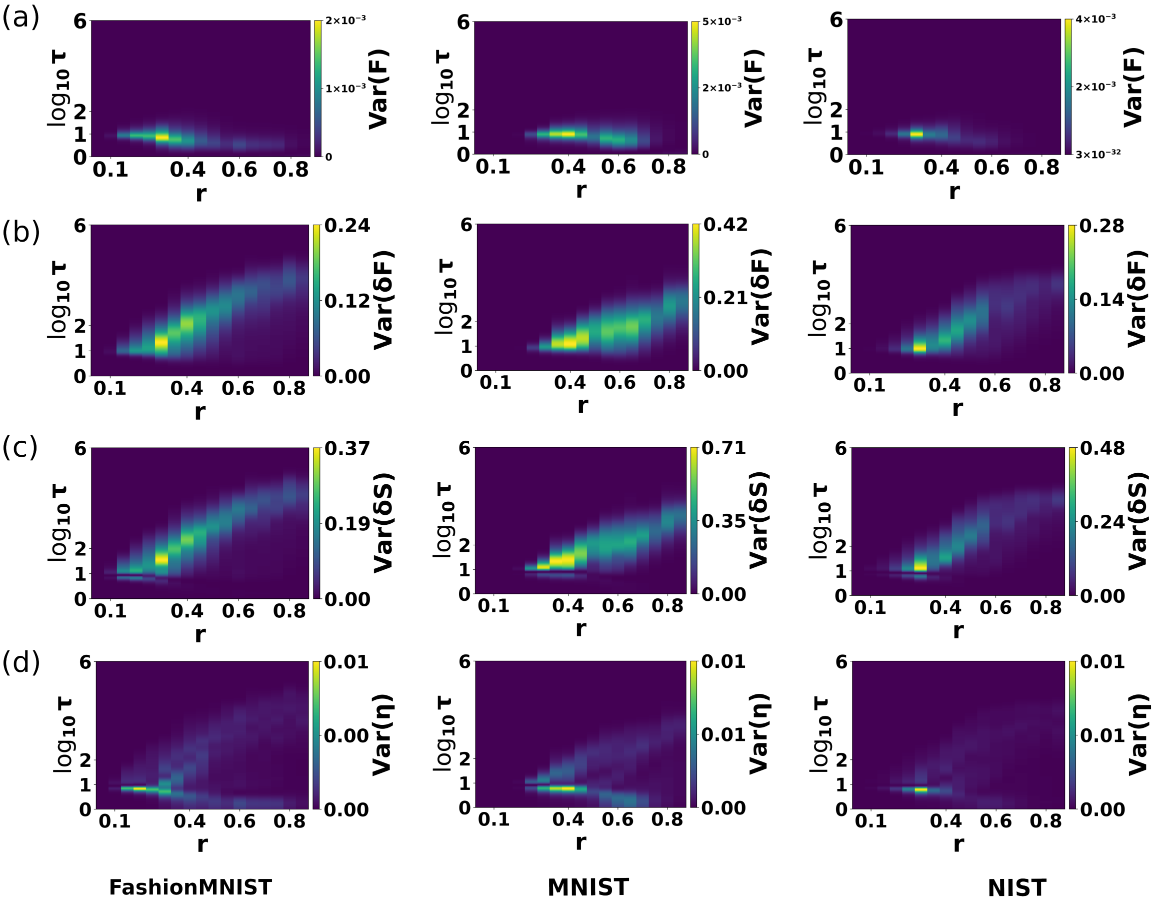


Figure S11: **Variance of F, $\delta$F, $\delta$S, $\eta$ - 2000 samples** in panels (a) through (d) for the three datasets (columns). The peaks of the variance indicate the structural phase transition. Variance computed over 50 independent simulations.

## S6 Variance analysis of $\hat{\mathrm{D}}$, $\hat{\mathrm{L}}$, and $S$

Figure S12 (for $N = 2000$) and Figure S13 (for $N = 4000$) show the following quantities. In panel (a) the ensemble degree $< \hat{D} >$, with lower bound $< \hat{D} >= 0$ for an isolated network and for $\tau \to \infty$ ; in panel (b) its variance. In panel (c) the internal energy, $U = \mathrm{Tr}[\hat{\rho}\hat{L}] =< \hat{L} >$, with $0 < U < 2|E|/N$ where the upper bound is given at $\tau = 0$, $U_{\tau=0} = \frac{1}{Z_{\tau=0}} \sum_i^N \lambda_i = \frac{2|E|}{N}$ while the lower bound for $\tau \to \infty$ or isolated nodes for all value of $\tau$; in panel (d) the variance of the internal energy. The color bar range is relative to the choice of the $\tau$ range illustrated. In panel (e) the variance of the von Neumann entropy, $S$. Note that $Var(S) \propto C$, where $C$ is the specific heat addressed in the main text.

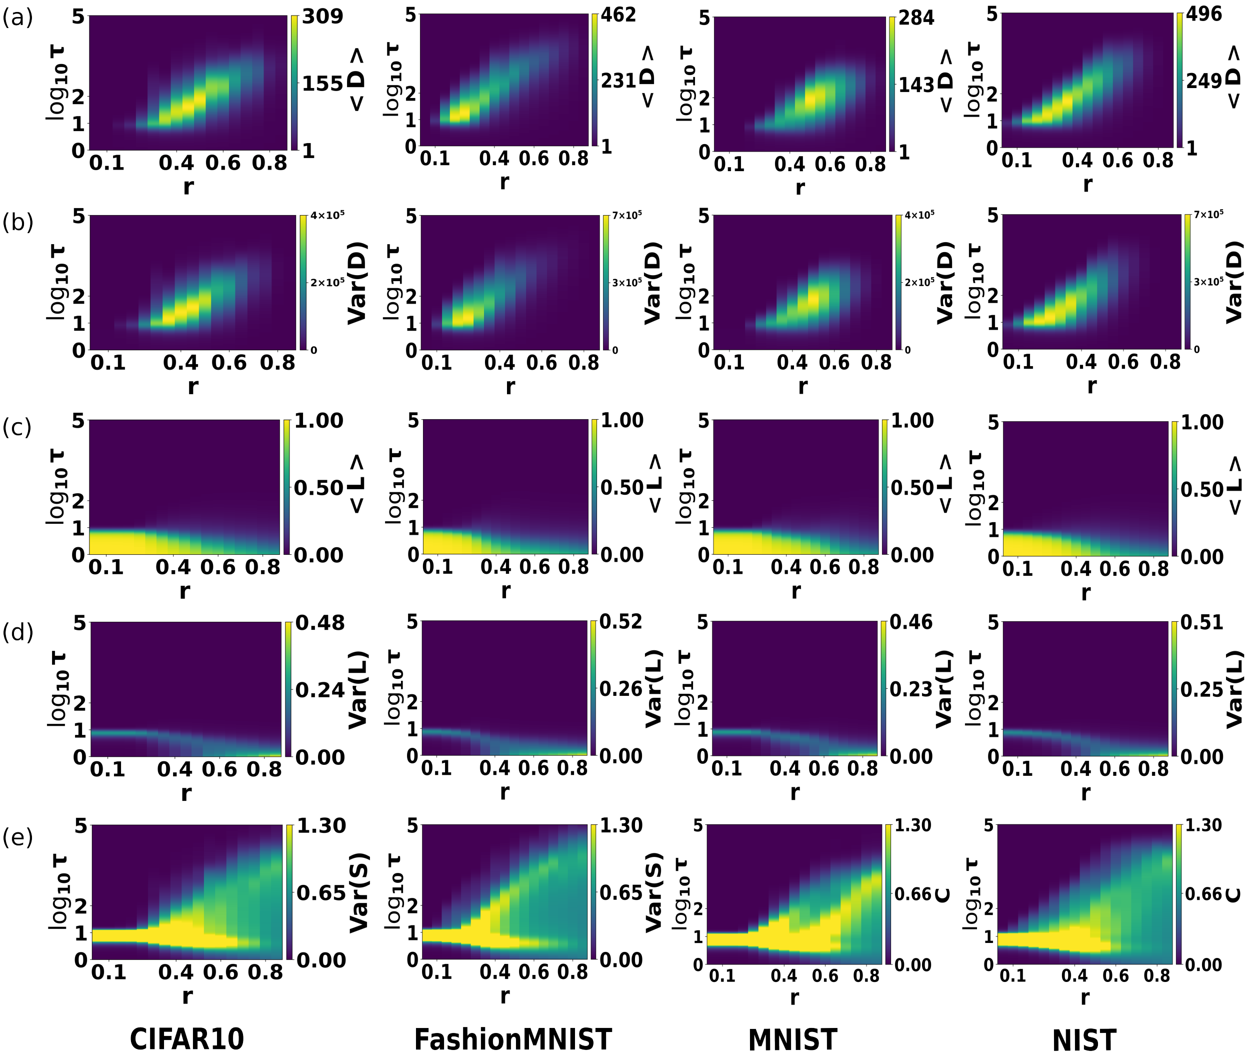


Figure S12: **Variance analysis of $\hat{\mathrm{D}}$, $\hat{\mathrm{L}}$, and $S$ - 2000 samples.** Panels (a) through (e) show $\hat{D}$, Var($\hat{D}$), $\hat{L}$, Var($\hat{L}$), and Var($S$), respectively. Notably, the contributions to the bifurcation of the specific heat ($C \propto$ Var($S$)) are disentangled by examining Var($\hat{D}$) and Var($\hat{L}$) in panels (b) and (d). In the main text, the quantity $U = \mathrm{Tr}[\hat{L}\hat{\rho}] = \langle\hat{L}\rangle$ is analyzed. Results are averaged over 50 simulations.

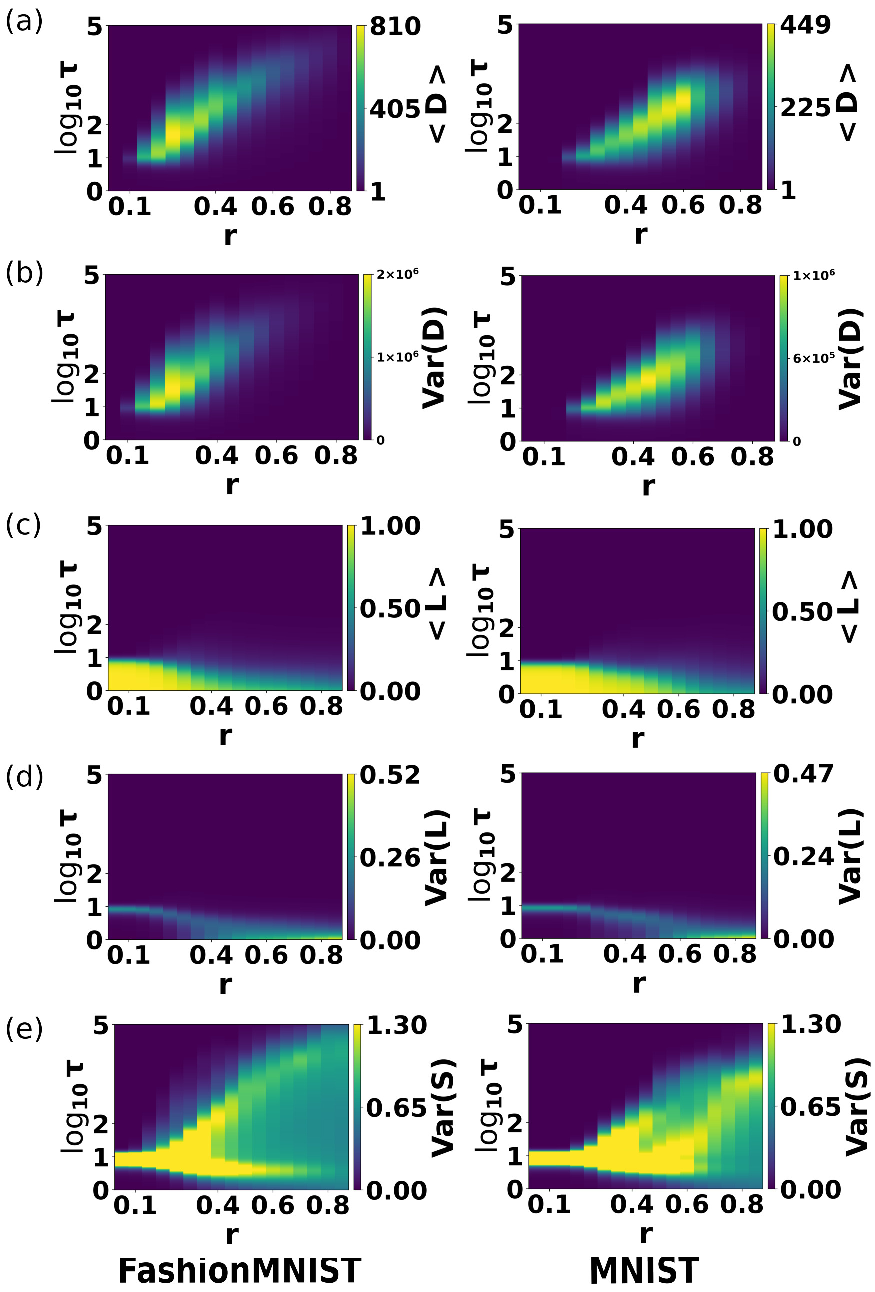


Figure S13: **Variance analysis of $\hat{\mathrm{D}}$, $\hat{\mathrm{L}}$, and $S$ - 4000 samples.** Panels (a) through (e) show $\hat{D}$, Var($\hat{D}$), $\hat{L}$, Var($\hat{L}$), and Var($S$), respectively. Notably, the contributions to the bifurcation of the specific heat ($C \propto$ Var($S$)) are disentangled by examining Var($\hat{D}$) and Var($\hat{L}$) in panels (b) and (d). In the main text, the quantity $U = \mathrm{Tr}[\hat{L}\hat{\rho}] = \langle \hat{L} \rangle$ is analyzed. Results are averaged over 50 simulations.

## S7 Pattern-matching efficiency

Figures S14 and S15 are produced by sampling samples from the MNIST (first row) and the FashionMNIST (second row). They show: the accuracy in panels (a)-(d); the (log)number of distances computed in panels (b)-(e); and the pattern-matching efficiency, $\theta$, in panels (c)-(f). Figure S14 shows results for 2000 samples drawn from the mentioned datasets, while Figure S15 shows results for 4000 samples.

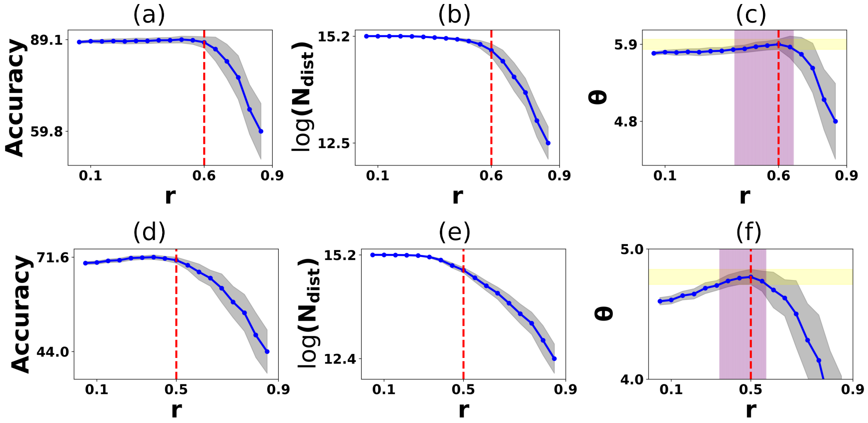


Figure S14: **Pattern-matching efficiency - 2000 samples** in **(c)-(f)** measured over the MNIST and FashionMNIST respectively. The pattern-matching efficiency, $\theta$, is defined as the ratio between the classification accuracy, **(a)-(d)**, and the logarithm of the number of distances computed to find the best match, **(b)-(e)**. The dashed-red vertical lines indicate the optimal $r$ value in terms of $\theta$. In each panel, the shaded grey area designates the standard deviation. The purple shaded area in panels **(c)-(f)** indicates a tolerance $r$-domain of optimal efficiency, $\theta$. The tolerance domain is defined as the $r$-values such that the corresponding $\theta$-values are included in one standard deviation computed at the maximum $\theta$, whose y-axis projection is indicated by the yellow shaded area. Curves are computed over 50 independent simulations with a subset of 2000 samples extracted from each dataset. The 10 classes are equally represented both in the train- and test sets.

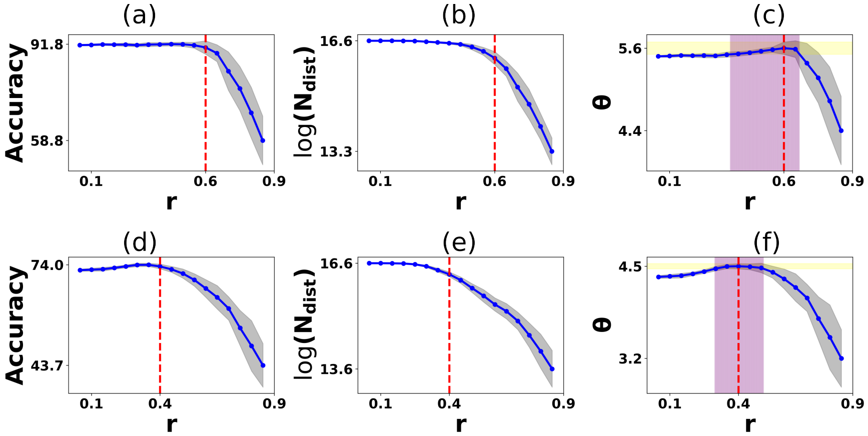


Figure S15: **Pattern-matching efficiency - 4000 samples** in **(c)-(f)** measured over the MNIST and FashionMNIST respectively. The pattern-matching efficiency, $\theta$, is defined as the ratio between the classification accuracy, **(a)-(d)**, and the logarithm of the number of distances computed to find the best match, **(b)-(e)**. The dashed-red vertical lines indicate the optimal $r$ value in terms of $\theta$. In each panel, the shaded grey area designates the standard deviation. The purple shaded area in panels **(c)-(f)** indicates a tolerance $r$-domain of optimal efficiency, $\theta$. The tolerance domain is defined as the $r$-values such that the corresponding $\theta$-values are included in one standard deviation computed at the maximum $\theta$, whose y-axis projection is indicated by the yellow shaded area. Curves are computed over 50 independent simulations with a subset of 4000 samples extracted from each dataset. The 10 classes are equally represented both in the train- and test sets.

## Author Contributions

DC: Theoretical framework, Conceptualization, Methodology, Simulations, Data curation, Software, Writing – original draft, Writing – review & editing. LS: Writing – review & editing, Conceptualization, Supervision, Funding acquisition.

## Funding

This work was funded by EUs Horizon 2020, from the MSCA-ITN-2019 Innovative Training Networks program ”Materials for Neuromorphic Circuits” (MANIC) under the grant agreement No. 861153, as well as by the financial support of the CogniGron research center and the Ubbo Emmius Funds (Univ. of Groningen).

## Acknowledgments

We are thankful to Jos van Goor for providing some of the scripts that enabled efficient grid-search across parameters and to Federico Balducci for the useful discussions.

## Data Availability Statement

The original contributions presented in the study are included in the article/supplementary material, further inquiries can be directed to the corresponding author/s. Datasets and scripts can be found at `https://github.com/CipolliniDavide/Laplacian_Trees`.
